# Supplementary material for: Boosting the Conformational Sampling by Combining Replica Exchange with Solute Tempering and Well-Sliced Metadynamics
Source: arXiv:2108.13641 source file (2021-08-31)
Supplement: Supplementary file 1 [file SI_GASS_Paper.pdf]

# Supporting Information for Boosting the Conformational Sampling by Combining Replica Exchange with Solute Tempering and Well-sliced Metadynamics

Anji Babu Kapakayala[†,‡] and Nisanth N. Nair[*,†]

†*Department of Chemistry, Indian Institute of Technology Kanpur, Kanpur 208016, India*

‡*School of Pharmacy and Biomedical Sciences, Curtin University, Perth WA 6845, Australia*

E-mail: nnair@iitk.ac.in

## 1 Collective Variables

### 1.1 Root mean squared deviation

The root mean squared deviation (RMSD), $\sigma^2_{\rm RMSD}$, of backbone $C_\alpha$ atoms with respect to the backbone $C_\alpha$ atoms (residues 1 - 15) of reference structure is defined as,

$$\sigma^2_{\rm RMSD} = \frac{\sum_I^N M_i(\mathbf{R}_I - \mathbf{R}_I^{\rm ref})^2}{\sum_I^N M_I} \tag{1}$$

Here, $N$ is the total number of $C_\alpha$ atoms, and $M_I$ is the mass of an atom $I$. Further, $\mathbf{R}_I$ and $\mathbf{R}_I^{\rm ref}$ are the coordinates of $C_\alpha$ atoms in a given structure and the reference structure, respectively.

## 1.2 Radius of gyration

The radius of gyration (Rg) of backbone $C_\alpha$ carbon atoms is calculated using,

$$\mathrm{Rg} = \sqrt{\frac{\sum_I^N M_I \left|\mathbf{R}_I - \mathbf{R}_{\mathrm{COM}}\right|^2}{\sum_I^N M_I}} \tag{2}$$

Here, $\mathbf{R}_{\mathrm{COM}} = \left(\sum_I^N \mathbf{R}_I M_I\right) / \left(\sum_I^N M_I\right)$ is the position of the center of the mass of the $C_\alpha$ carbon atoms.

## 1.3 $\alpha$-Helicity

$\alpha$-Helicity coordinate is defined as,

$$\mathrm{A_h} = \frac{1}{2} \sum_I \left[1 + \cos(\chi_I - \chi_I^{\mathrm{ref}})\right] \tag{3}$$

where $\chi_I$ are the instantaneous values for the Ramachandran angles, where we used $\phi^{\mathrm{ref}}$ $=-1.0$ and $\psi^{\mathrm{ref}}$$=-0.82$ radians, following Pfaendtner et. al.[1]

# 2 Conformational Free Energy Landscape of Trp-Cage for Various Simulation Lengths

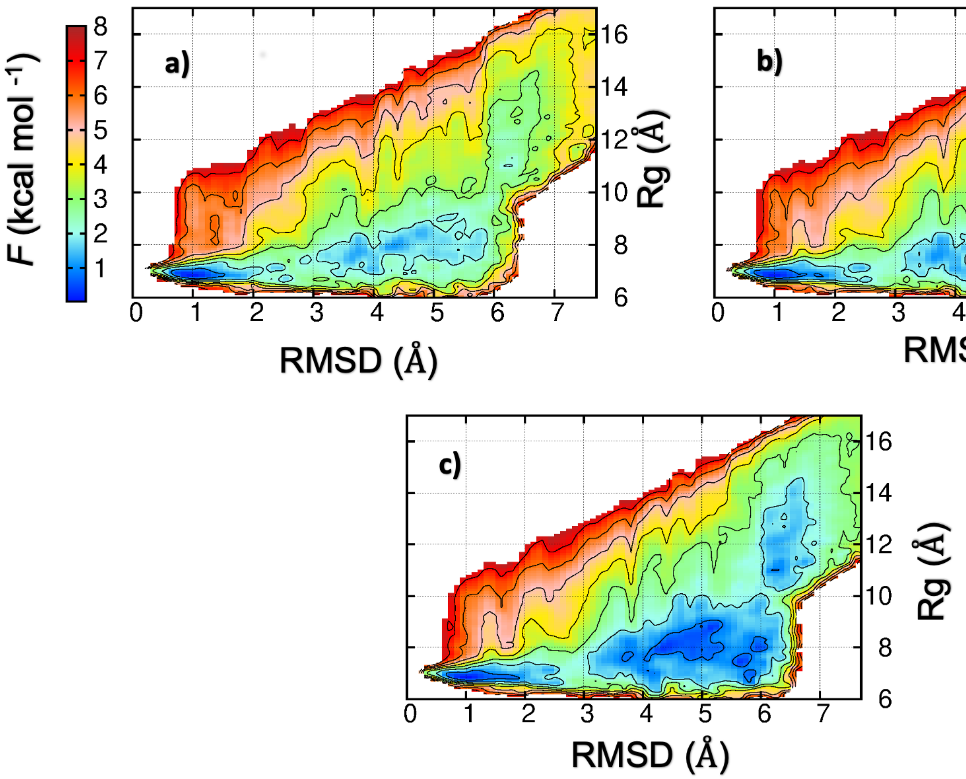


Figure 1: Free energy surface reconstructed as a function of RMSD and Rg from GASS simulations after (a) 50 ns, (b) 75 ns, and (c) 100 ns.

# 3 Derivation of Exchange Probability for GASS

Acceptance ratio for the exchange of replicas $i$ and $j$ is given by $\exp(-\Delta_{i,j})$ where[2]

$$\Delta_{i,j} = -\beta_i \left[ U_i(\mathbf{R}_j) - U_i(\mathbf{R}_i) \right] - \beta_j \left[ U_j(\mathbf{R}_i) - U_j(\mathbf{R}_j) \right] \ . \tag{4}$$

In GASS and REST2[3] the temperature of the replicas $i$ and $j$ are the same. Thus,

$$\beta_i = \beta_j = \beta_0 \ . \tag{5}$$

Potential energy function $U$ for GASS is given by,

$$U_i^{\rm GASS}(\mathbf{R}) = U_i^{\rm REST2}(\mathbf{R}) + V_i^{\rm b}\left(s(\mathbf{R}),t\right) + W_i^{\rm b}\left(s(\mathbf{R})\right), \ \ h=1,\cdots,M, \tag{6}$$

and[3]

$$U_i^{\rm REST2}(\mathbf{R}) = \frac{\beta_i}{\beta_0}U_{\rm pp}(\mathbf{R}) + \sqrt{\frac{\beta_i}{\beta_0}}U_{\rm pw}(\mathbf{R}) + U_{\rm ww}(\mathbf{R}) \ \ . \tag{7}$$

In the above, $U_{\rm pp}$, $U_{\rm pw}$, and $U_{\rm ww}$ are potential energy functions for protein-protein, protein-water, and water-water interactions.[3] On substituting Eq. (5), Eq. (6), and Eq. (7) in Eq. (4) yields

$$\Delta_{i,j} = \Delta_{i,j}^{(1)} + \Delta_{i,j}^{(2)} \tag{8}$$

where

$$\Delta_{i,j}^{(1)} = (\beta_i - \beta_j)\left[(U_{\rm pp}(\mathbf{R}_j) - U_{\rm pp}(\mathbf{R}_i)) + \frac{\sqrt{\beta_0}}{\sqrt{\beta_i}+\sqrt{\beta_j}}(U_{\rm pw}(\mathbf{R}_j) - U_{\rm pw}(\mathbf{R}_i))\right] \ \ , \tag{9}$$

and

$$\Delta_{i,j}^{(2)} = \beta_0\left\{\left[V_i^{\rm b}(\mathbf{s}_j,t) - V_i^{\rm b}(\mathbf{s}_i,t)\right] - \left[V_j^{\rm b}(\mathbf{s}_j,t) - V_j^{\rm b}(\mathbf{s}_i,t)\right]\right\} \ \ . \tag{10}$$

Since the umbrella potential acting on the replicas $i$ and $j$ has the same functional form, they cancel each other and therefore all the terms involving $W^{\rm b}$ are cancelled out.

# 4 Other Intermediate Structures

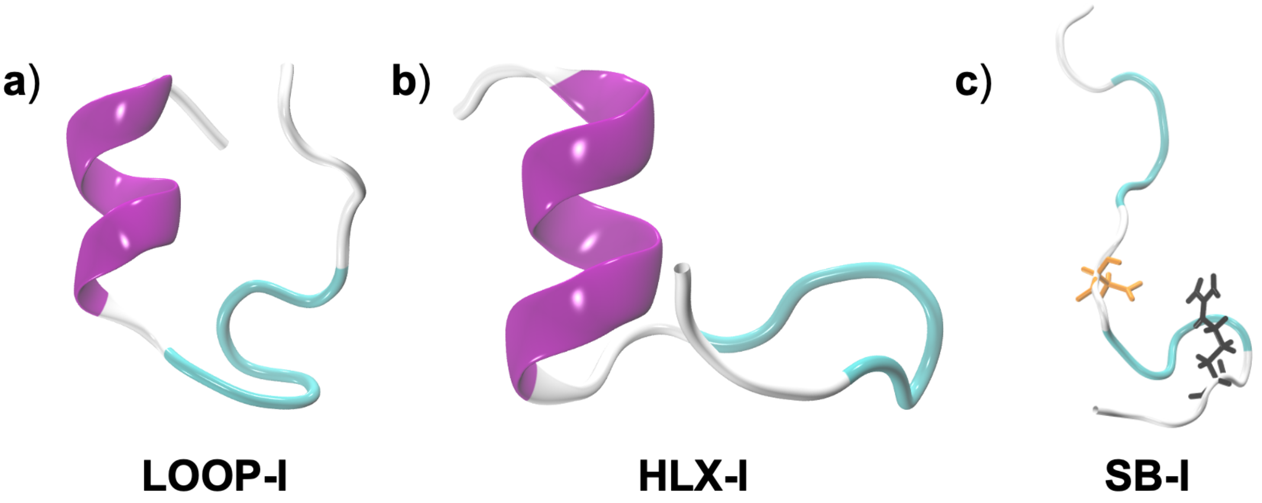


Figure 2: Intermediate structures observed in the GASS simulation trajectories which resembled (a) LOOP-I, (b) HLX-I, and (c) SB-I intermediates reported by Kim et al.[4]

# References


(1) Pfaendtner, J.; Bonomi, M. *J. Chem. Theory Comput.* **2015**, *11*, 5062–5067.

(2) Liu, P.; Kim, B.; Friesner, R. A.; Berne, B. J. *Proc. Nat. Acad. Sci.* **2005**, *102*, 13749–13754.

(3) Wang, L.; Friesner, R. A.; Berne, B. J. *J. Phys. Chem. B* **2011**, *115*, 9431–9438.

(4) Kim, S. B.; Dsilva, C. J.; Kevrekidis, I. G.; Debenedetti, P. G. *J. Chem. Phys.* **2015**, *142*, 085101.
